# Supplementary material for: Towards a responsible machine learning approach to identify forced labor in fisheries
Source: arXiv:2302.10987 ancillary file (2023-02-03)
Supplement: Supplementary file 1 [file Supp1.pdf]

# Title and abstract in multiple languages

## English version

### Towards a responsible machine learning approach to identify forced labor in fisheries

Many fishing vessels use forced labor, but identifying vessels that engage in this practice is challenging because few are regularly inspected. We developed a positive-unlabeled learning algorithm using vessel characteristics and movement patterns to estimate an upper bound of the number of positive cases of forced labor, with the goal of helping make accurate, responsible, and fair decisions. 89% of the reported cases of forced labor were correctly classified as positive (recall) while 98% of the vessels certified as having decent working conditions were correctly classified as negative. The recall is high for vessels from different regions using different gears, except for trawlers. We found that as much as ~28% of vessels may operate using forced labor, with the fraction much higher in squid jiggers and longlines. This model could inform risk-based port inspections as part of a broader monitoring, control, and surveillance regime to reduce forced labor.

## Spanish version

### Hacia un uso responsable del aprendizaje automático para identificar el trabajo forzoso en pesquería

Numerosas embarcaciones pesqueras utilizan mano de obra forzada, pero resulta difícil identificar a los buques que utilizan esta práctica, ya que son pocos los que se inspeccionan con regularidad. Desarrollamos un algoritmo de aprendizaje de tipo positive-unlabeled que utiliza las características de los buques y los patrones de movimiento para obtener una estimación máxima de casos positivos de trabajo forzoso, con el objetivo de ayudar a tomar decisiones precisas, responsables y justas. El 89% de los casos de trabajo forzoso notificados se clasificaron correctamente como positivos (recall), mientras que el 98% de las embarcaciones certificadas con condiciones de trabajo decentes se clasificaron correctamente como negativas. El valor de recall es alto en los buques de diferentes regiones que utilizan diferentes artes, excepto para los arrastreros. Descubrimos que hasta un 28% de las embarcaciones pueden trabajar con mano de obra forzada, y que esta proporción es mayor en

la pesca de calamar con poteras y los palangreros. Este modelo podría servir de base para las inspecciones portuarias basadas en riesgo como parte de un régimen más amplio de seguimiento, control y vigilancia para reducir el trabajo forzoso.

## French version

### Vers une approche responsable de l'apprentissage automatique pour identifier le travail forcé dans la pêche

De nombreux navires de pêche ont recours au travail forcé, mais l'identification des navires qui se livrent à cette pratique est difficile car peu d'entre eux sont régulièrement inspectés. Nous avons développé un algorithme d'apprentissage automatique de type positif-non étiqueté utilisant les caractéristiques des navires et les patterns de mouvement pour estimer une limite supérieure du nombre de cas positifs de travail forcé, dans le but d'aider à la prise de décisions fiables, responsables et justes. 89 % des cas de travail forcé rapportés ont été correctement classés comme positifs (rappel), tandis que 98 % des navires certifiés comme ayant des conditions de travail décentes ont été correctement classés comme négatifs. Le taux de rappel est élevé pour les navires de différentes régions utilisant différents engins de pêche, à l'exception des chalutiers. Nous avons constaté que jusqu'à ~28% des navires pourraient opérer en utilisant le travail forcé, avec une fraction beaucoup plus élevée dans la pêche à la turlutte et les palangriers. Ce modèle pourrait servir de base aux inspections portuaires orientées sur le risque dans le cadre d'un régime plus large de suivi, contrôle et surveillance visant à réduire le travail forcé.

## Simplified Chinese version

### 建立一个负责任的机器学习方法来识别渔业中的强迫劳动

强迫劳动存在许多渔船上，由于很少有船只被定期检查，识别涉及强迫劳动的船只具有挑战性。我们开发了一种正面未标记的学习算法，使用船只的特征和运动模式来估计强迫劳动的正面案例数量的上限，目的是帮助做出准确、负责任和公平的决策。89%的强迫劳动报告案例被正确地归类为正面案例（召回率），而98%被认证为具有合宜工作条件的船只被正确地归类为负面案例。除拖网渔船外，不同地区使用不同渔具的船只的召回率都很高。我们发现，多达28%的船只可能存在强迫劳动，其中鱿鱼钓船和延绳钓船的比例要高得多。这个模型可以为基于风险的港口检查提供信息，作为更广泛的监测、控制和监督制度的一部分，以减少强迫劳动。

## Traditional Chinese version

### 建立一個負責任的機器學習方法識別漁業中的強迫勞動

強迫勞動存在許多漁船上，由於很少船隻被定期檢查，識別涉及強迫勞動的船隻具有挑戰性。我們開發了一種正面未標記的學習演算法，使用船隻的特徵和作業模式來估算強迫勞動的正面案例數量的上限，其目的是幫助做出準確、負責任和公平的決策。89%的強迫勞動報告案例被正確地歸類為正面案例（召回率），而98%被證實為具有合宜工作條件的船隻被正確地歸類為負面案例。除拖網漁船外，不同地區使用不同漁具的船隻的召回率都很高。我們發現，多達28%的船隻可能存在強迫勞動，其中魷釣船和延繩釣船的比例要高得多。這個模型可以為基於風險管理的港口檢查提供資訊，作為更廣泛的監測、管制與偵察制度的一部分，以減少強迫勞動。

## Indonesian version

### Menuju pendekatan pembelajaran mesin (machine learning) yang bertanggung jawab untuk mengidentifikasi kerja paksa dalam perikanan

Tercatat banyak kapal penangkap ikan yang menggunakan metode kerja paksa pada awak kapalnya, tetapi mengidentifikasi kapal yang terlibat dalam praktik ini cukup sulit karena hanya sedikit yang diperiksa secara rutin. Kami mengembangkan algoritma pembelajaran tanpa label positif (a positive-unlabeled learning algorithm) menggunakan karakteristik kapal dan pola pergerakan untuk memperkirakan batas atas jumlah kasus positif kerja paksa, dengan tujuan membantu membuat keputusan yang akurat, bertanggung jawab, dan adil. 89% dari kasus-kasus kerja paksa yang dilaporkan diklasifikasikan sebagai positif (recall), sementara 98% kapal yang disertifikasi memiliki kondisi kerja yang layak diklasifikasikan sebagai negatif. "Recall" dikategorikan cukup tinggi untuk kapal-kapal dari berbagai wilayah yang menggunakan alat tangkap yang berbeda, kecuali kapal pukat. Kami menemukan bahwa sebanyak ~28% kapal mungkin beroperasi dengan menggunakan metode kerja paksa pada awaknya, dengan fraksi yang jauh lebih tinggi pada kapal pukat cumi dan rawai. Model ini dapat menginformasikan pihak inspeksi pelabuhan untuk melakukan pemeriksaan berbasis risiko sebagai bagian dari kebijakan pemantauan, pengendalian, dan pengawasan yang lebih luas untuk mengurangi kerja paksa.
