# Supplementary material for: Towards a responsible machine learning approach to identify forced labor in fisheries
Source: arXiv:2302.10987 ancillary file (2023-02-03)
Supplement: Supplementary file 2 [file Supp2.pdf]

# Towards a responsible machine learning approach to identify forced labor at sea - Supplementary File

## Sensitivity analyses and model calibration

To choose the number of times to downsample the training sets in each split (here called bags), the hyperparameters of the random forests (RFs), and the number of seeds, we performed sensitivity analysis and model calibration procedures described in this section.

### Bags

To choose the number of bags, we aimed for a stable area under the ROC curve (AUC) from the RFs (fitted in step 2 in the model described in the main text). AUC was the chosen performance metric because it has shown to be robust to corrupted binary labels—as in our case because the positively labeled cases have not been collected through representative unbiased sampling.

For this analysis, we used only one initial seed and fixed RF hyperparameter values:  $mtry = 3$ ,  $min_n = 20$ , and  $regularization.factor = 0.788$ . We will describe these parameters in the next section; the values used in this test provided optimal results in previous versions of the model. We then assumed that a 30-bag configuration would provide accurate AUC and aimed to identify a lesser amount of bags that would lead to a similar AUC. Therefore, we started with a 30-bag configuration and computed AUC. Then, the 30-bag dataset (that contained predictions with the 30 RFs), was split into three groups of 10-bag datasets and AUC was computed for each of these groups. The 30-bag dataset was also split into six groups of five bags and 30 groups of one bag. AUC was computed for each group of 1, 5, 10, and 15 bags configurations and then compared to the 30-bag-configuration AUC.

AUC is fairly stable for 10 bags (Fig. 1), so we chose 10 bags for the model.

### RF hyperparameters

Three RF hyperparameters were calibrated: the number of features used to split on at each node ( $mtry$ ), the minimum number of vessel-years that a final node should have ( $min_n$ ), and the regularization factor (regularization works by penalizing new variables by multiplying the splitting criterion by a factor). A grid of 630 combinations of  $mtry$ ,  $min_n$ , and regularization factor values was generated with 10 values of  $mtry$  (from 1 to 10), 7 values of  $min_n$  (from 10 to 40, increasing by 5), and 9 values of regularization factor (from 0.1 to 0.9, increasing by 0.1).

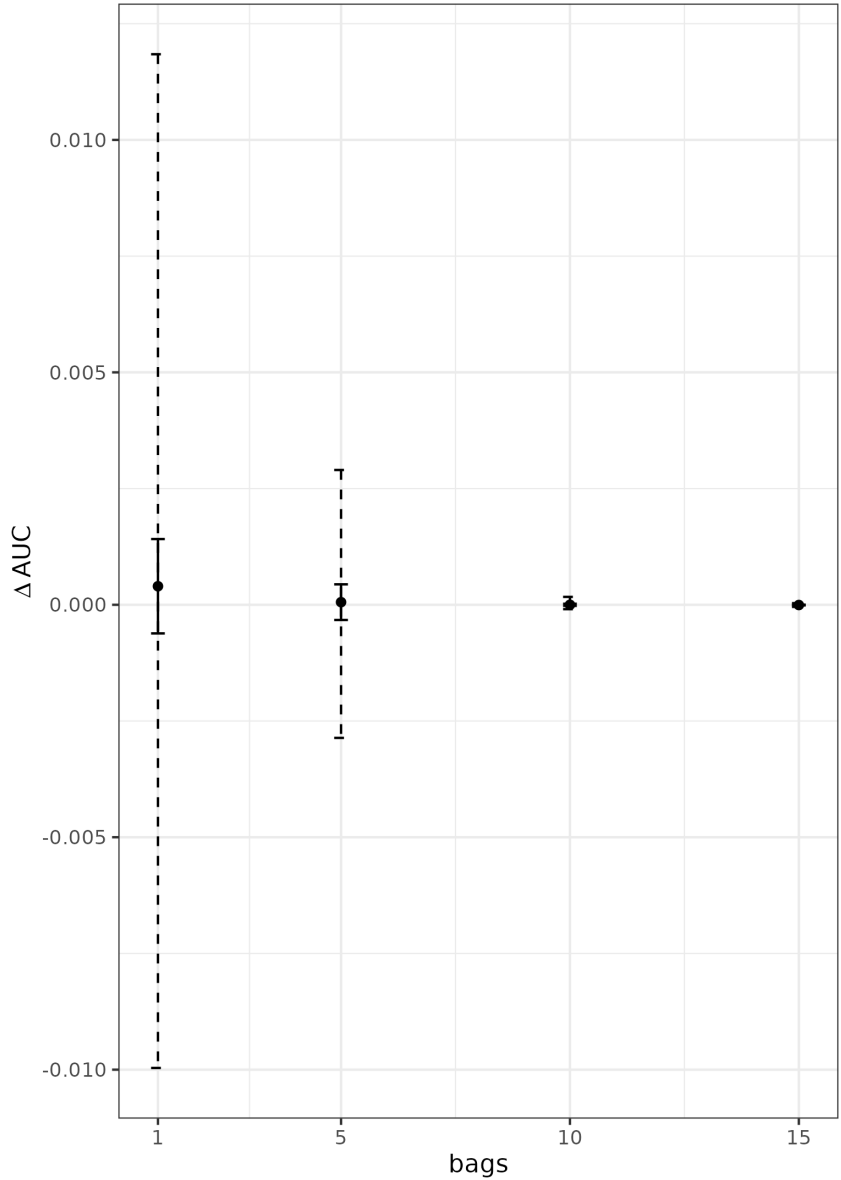

Figure 1: Difference in AUC between a 30-bag configuration random forest algorithm and 1, 5, 10, and 15 bags configurations. The black dots correspond to the average difference, the solid bars correspond to the average plus/minus the standard deviation, and the dashed bars correspond to the maximum and minimum difference.

We chose the hyperparameter combination that attained the highest AUC—like in the previous section, corresponding to step 2 in the model described in the main text, and using one seed and 10 bags. This combination was  $mtry = 1$ ,  $min_n = 15$ , and regularization factor = 0.5. AUC is flat near the optimum (Fig. 2), showing that the model is not too sensitive to the choice of hyperparameters; see Fig. 3 for a complete picture of the results.

## Seeds

With a chosen number of bags and RF hyperparameter values, we tested the sensitivity of global model outcomes, i.e. alpha, recall, and specificity, to changes in

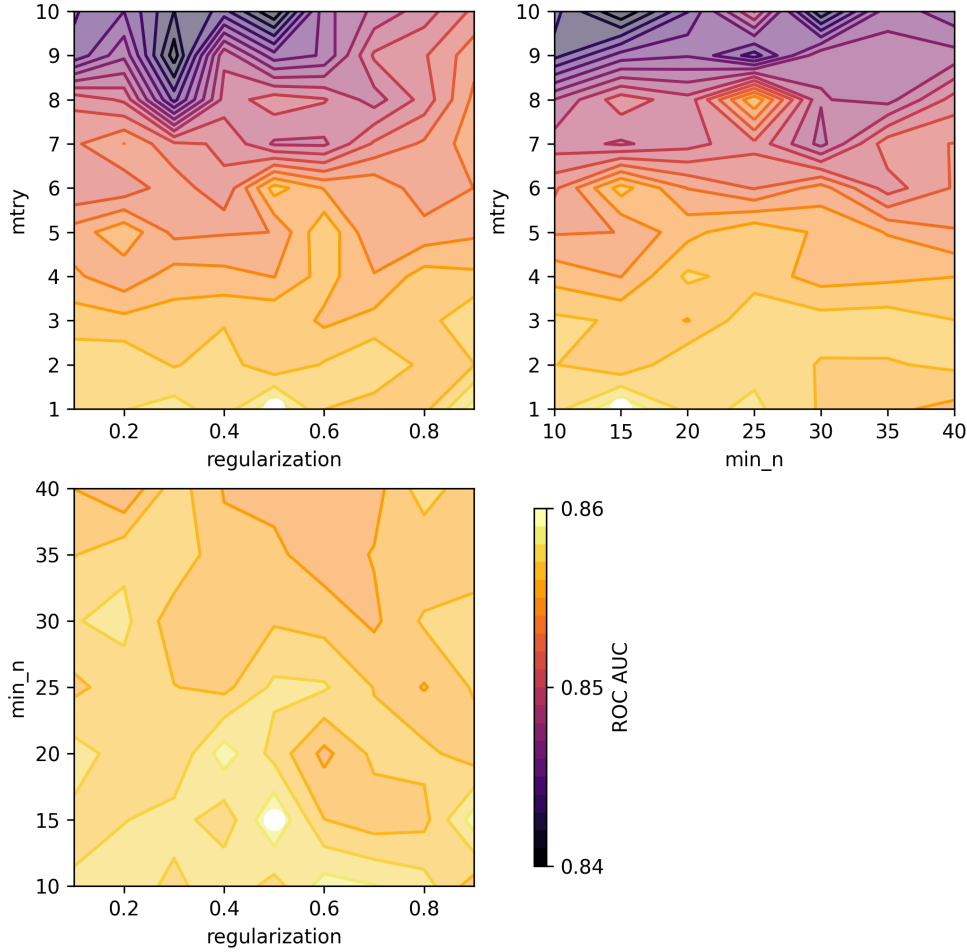

Figure 2: Contour lines and colors for AUC values for combinations of  $mtry$  and regularization factor when  $min_n = 15$  (top left), combinations of  $mtry$  and  $min_n$  when regularization factor = 0.5, and for combinations of  $min_n$  and regularization factor when  $mtry = 1$ . The white dot represents the combination with the highest AUC.

the number of initial seeds. We then assumed that a 15-seed configuration would provide accurate alpha, recall, and specificity values, and aimed to identify a lesser amount of seeds that would lead to similar outcomes. Therefore, we started with a 15-seed configuration, fitted the whole model, and computed the three metrics. Then, the 15-seed dataset was split into three groups of five-bag datasets, fitted the model, and the metrics were computed for each of these three groups. The 30-bag dataset was also split into five groups of three seeds and 15 groups of one seed. Alpha, recall, and specificity were computed for each group and then compared to the 15-seed model metrics.

The three metrics are fairly stable for three seeds (Fig. 4), so we chose three seeds for the model.

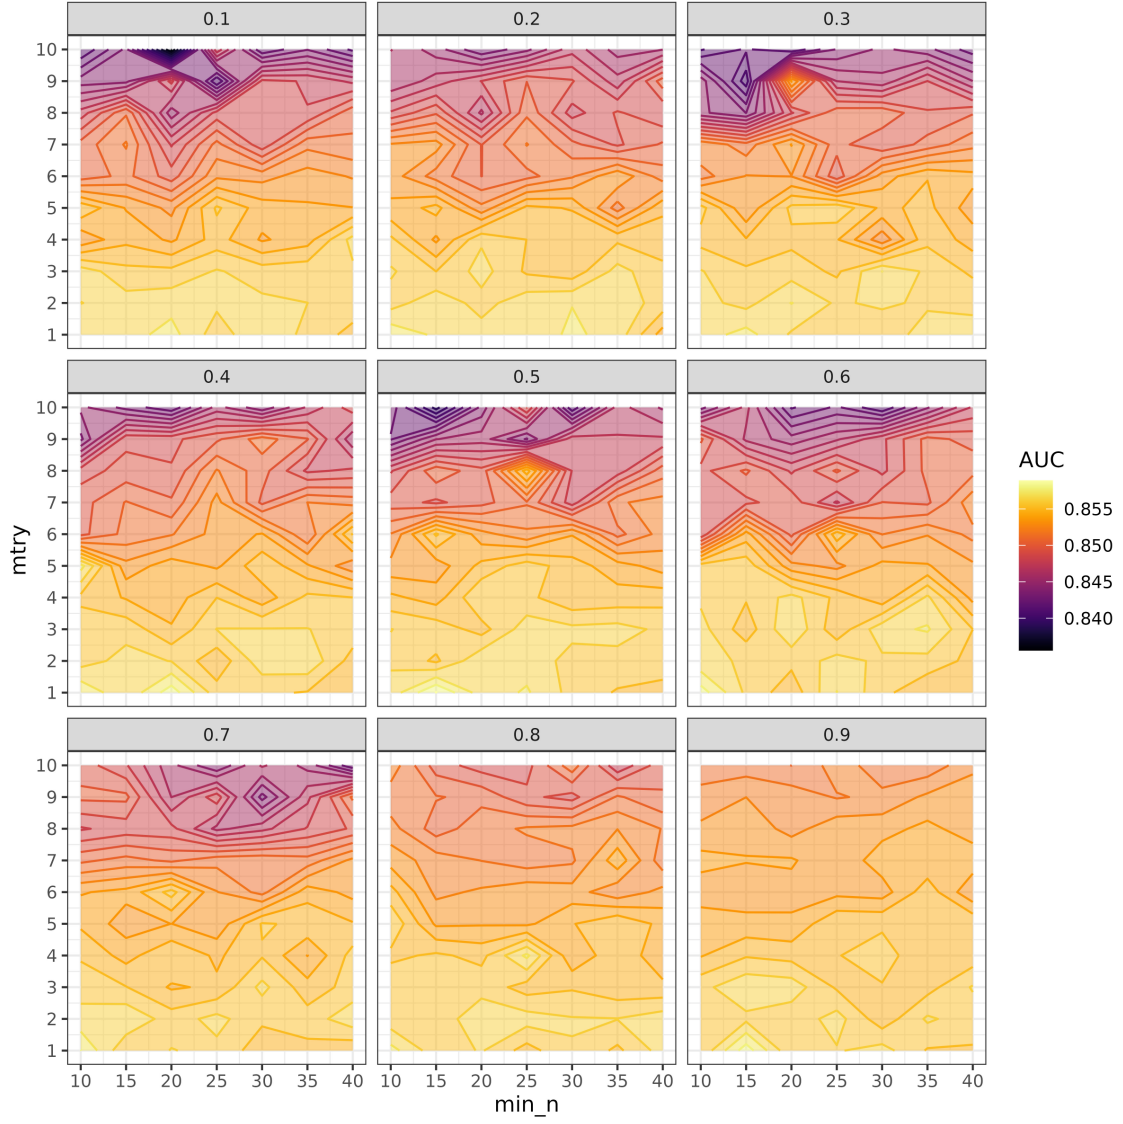

Figure 3: Contour lines and colors for AUC values for all combinations of  $mtry$  and  $min_n$  for each regularization factor value.

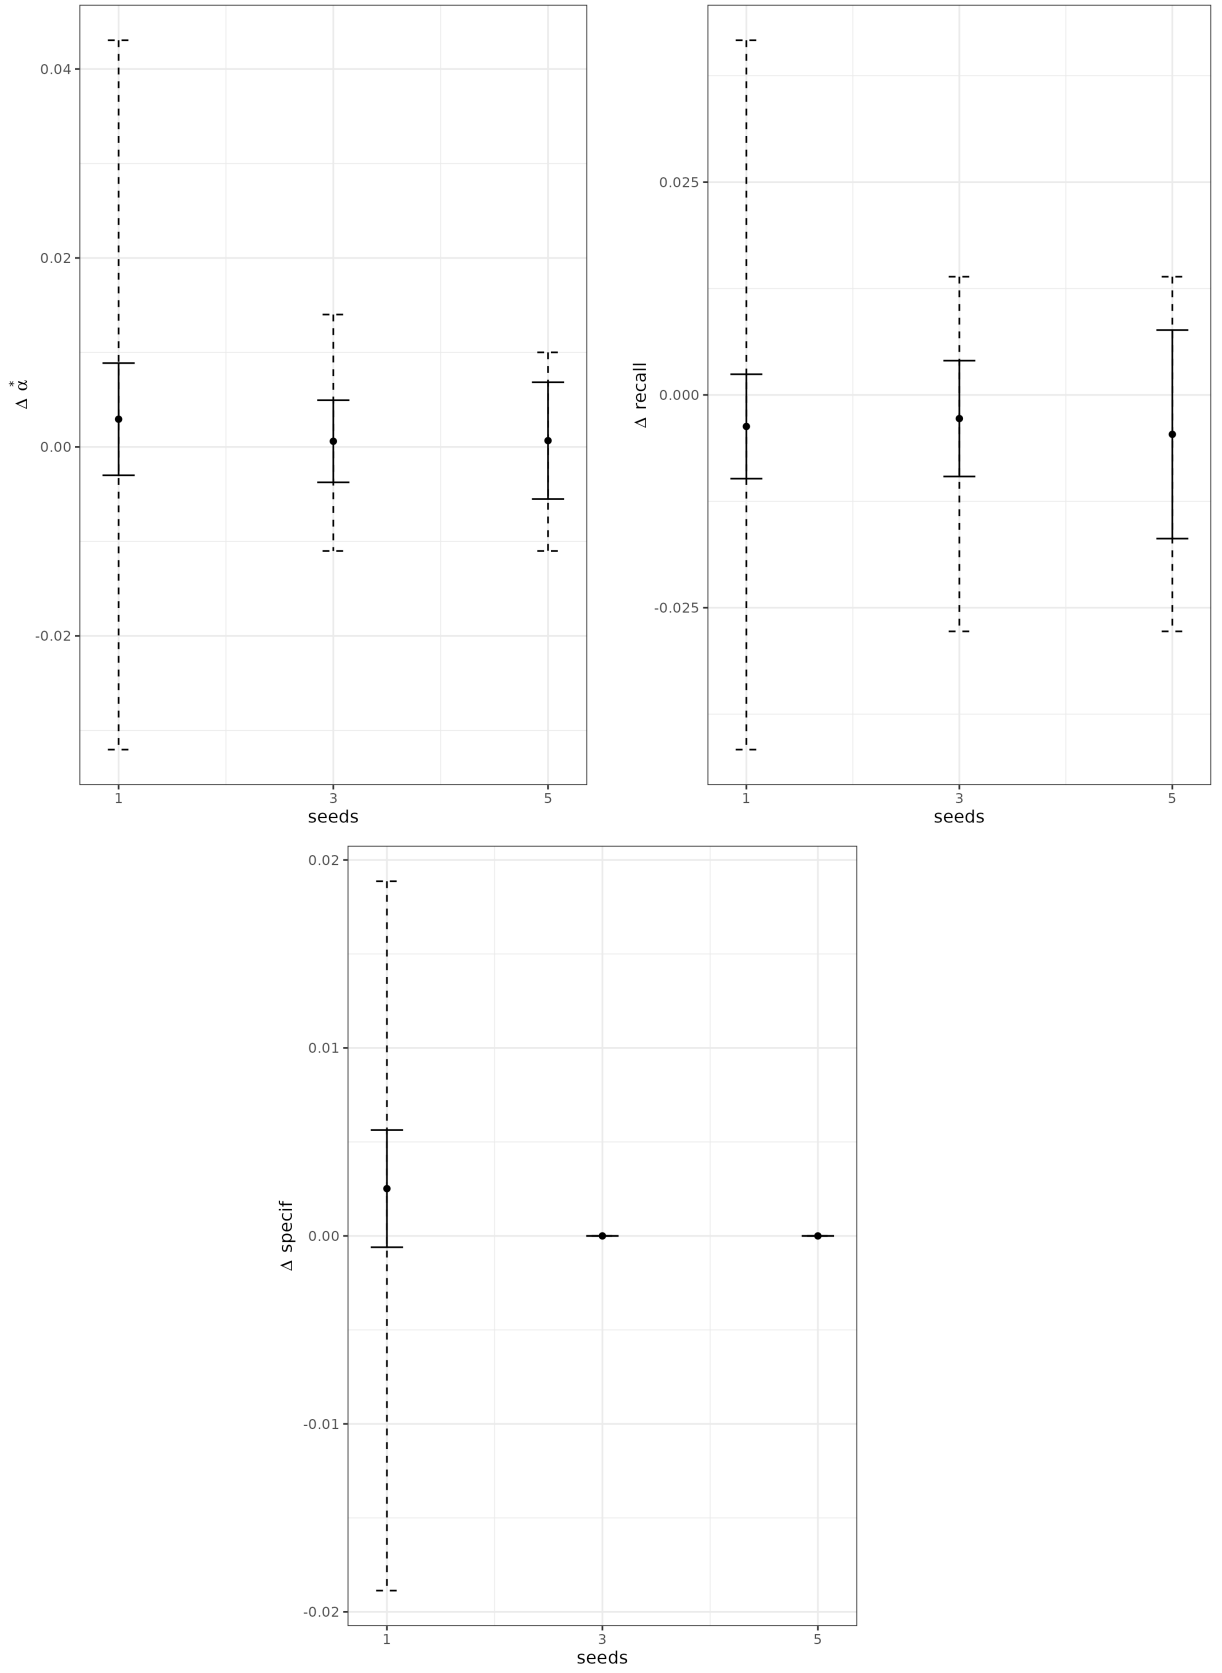

Figure 4: Difference in alpha (top left), recall (top right), and specificity (bottom) between a 15-seed model and 1, 3, and 5-seed models. The black dots correspond to the average difference, the solid bars correspond to the average plus/minus the standard deviation, and the dashed bars correspond to the maximum and minimum difference.
